# Supplementary material for: Demystifying Orthogonal Monte Carlo and Beyond
Source: arXiv:2005.13590 source file (2020-05-27)
Supplement: Supplementary file 1 [file additional.tex]

\section{Extra material not included in main}
\label{sec:additional}

Let's consider $F_f(Z)=E_{\omega \in \mathcal{D}}[f(|\omega^T Z|)]$ where we assume $f: \mathcal{R}^{+} \mapsto \mathcal{R}$ can be expressed as Taylor series expending at zero with remaining term satisfying $\lim_{N \to \infty} R_N(x)=0$. The standard Monte Carlo estimator samples independently $\omega_i^{iid} \sim \mathcal{D}$, and then averages these samples over $i$: $\hat{F}_m^{iid}(Z)=\frac{1}{m} \sum_{i=1}^m f(|{\omega_i^{iid}}^T Z|)$, while the orthogonal estimator samples $\omega_i^{ort} \bot \omega_j^{ort}, \forall i \neq j $, and then averages over $i$: $\hat{F}_m^{ort}(Z)=\frac{1}{m} \sum_{i=1}^m f(|{\omega_i^{ort}}^T Z|)$. These orthogonal vectors can be constructed by performing Gram-Schimidt orthogonalization and then renormalizing the rows such that the length of the renormalized row is sampled from the
distribution from which $\Vert \omega_i^{iid} \Vert s$ are sampled. Both of these two estimators are trivially unbiased.

Now, let's explain how to utilize properties from negative association to prove that orthogonal random features can achieve better strong concentration bound than independent random features. 

Firstly, by applying Markov Inequality to some monotone functions, we can derive the following lemma.

\begin{lem} [Extended Markov Inequality] \label{Lem_ExtendedMarkovInequality} 
If $D(X)$ is a non-increasing and non-negative function for all $X \geq 0$, and $I(X)$ is a non-decreasing and non-negative function for all $X \geq 0$. Then $\forall X \geq 0, \forall k > 0 $, we have:
$$ P(X \geq k) = P(I(X)\geq I(k)) \leq \frac{E[I(X)]}{I(k)}$$
$$ P(X \leq k) = P(D(X)\geq D(k)) \leq \frac{E[D(X)]}{D(k)}$$
\end{lem}

We can apply Lemma \ref{Lem_ExtendedMarkovInequality} to our problem to get the concentration bound
$P( \hat{F}_{m} \geq a)\leq \frac{E[I(\hat{F}_{m}]}{I(a)} $ and 
$P( \hat{F}_{m} \leq a)\leq \frac{E[D(\hat{F}_{m}]}{D(a)} $ hold for both independent samples $\hat{F}_{m}^{iid}$ and orthogonal samples $\hat{F}_{m}^{ort}$, and $\forall a > 0$. If the orthogonal samples have better concentration bound than iid samples, then we should have
$ {E[I(\hat{F}^{ort}_{m})]} \leq {E[I(\hat{F}^{iid}_{m})]} $ and 
$ {E[D(\hat{F}^{ort}_{m})]} \leq {E[D(\hat{F}^{iid}_{m})]} $.

As for the specific form of $D(X)$ and $I(X)$, we can use exponential functions in order to transform the products of $m$ samples into summations. So we define $I(x)=\mathrm{e}^{\theta mx}$ and $D(x)=\mathrm{e}^{-\theta mx}$, where $\theta \geq 0$. Since $\hat{F}_{m}=\frac{1}{m}\sum_{i=1}^{m}X_{i}$, the equivalent inequality we need to prove can be written as
$ E[ \mathrm{e}^{ \theta\sum_{i=1}^{m}X_{i}^{ort} } ] \leq E[ \mathrm{e}^{ \theta \sum_{i=1}^{m}X_{i}^{iid} } ] = \prod_{i=1}^{m} E[\mathrm{e}^{\theta X_{i}^{iid} } ] $, and $ E[ \mathrm{e}^{ -\theta\sum_{i=1}^{m}X_{i}^{ort} } ] \leq E[ \mathrm{e}^{- \theta \sum_{i=1}^{m}X_{i}^{iid} } ] = \prod_{i=1}^{m} E[\mathrm{e}^{-\theta X_{i}^{iid} }]$.
If we combine these two inequalities, then we actually need to prove that
$ E[ \mathrm{e}^{ \lambda \sum_{i=1}^{m}X_{i}^{ort} } ] \leq \prod_{i=1}^{m} E[\mathrm{e}^{\lambda X_{i}^{iid} } ]$, Where $\lambda$ can take both positive and negative values.

Next, we first deviate from our proof by introducing the concepts of negative association (NA) and negative dependence (ND) from \cite{Wajc217,Joag-Dev183}, and then prove that $X_1^{ort},…,X_n^{ort}$ satisfy ND.

\begin{definition}[Negative Association (NA)] \label{Def_NA} 
A set of random variables $X_1,…,X_n$ is said to be negatively associated (NA) if for any two disjoint index sets $I,J \subseteq [n]$, and two functions $f and g$ either both non-decreasing or both non-increasing, it holds: $ E( f(X_i:i\in I) g(X_j:j\in J) ) \leq E(f(X_i:i\in I)) E(g(X_j:j\in J)) $ 
\end{definition}

\begin{lem} \label{Lem_appendix2}
Let $I_1,...,I_n$ be disjoint subsets of $\{1,...,k\}$ and $f_1,…,f_n$ be non-decreasing (non-increasing) positive functions. Then $X_1,…,X_k$ NA implies:
$$ E[\prod_{i=1}^{n} f_i(X_j:j\in I_i)] \leq \prod_{i=1}^n E[f_i(X_j: j \in I_i )]  $$
\end{lem}

Lemma \ref{Lem_NA_ExpectationProductInequality} can be proved by Definition 1 by induction. 
For $k=2$, we have already know it from Definition \ref{Def_NA}.
Assume that this holds for $k=m-1$. $ E[\prod_i^{m-1} f_i(X_j:j\in I_i)] \leq \prod_i^{m-1} E[f_i(X_j: j \in I_i )] $
For $k=m$, since the product of two monotone non-decreasing functions will also be monotone non-decreasing, so we can define $ f_{1:m-1} = \prod_i^{m-1} E[f_i(X_i: i \in I_i )] $, which will still be a monotone non-decreasing function defined on the union of the index sets of $X_1,…,X_{m-1}$, and this union set is also disjoint with the index set formed by $X_m$. And by using Definition \ref{Def_NA} and the assumption we made in the case $k=m-1$, Lemma \ref{Lem_NA_ExpectationProductInequality} can be proved. 

\begin{corollary} \label{Cor_NA_ProbabilityInequality}
If $X_1,…,X_n$ are NA random variables, then for any set of values $x_1,…,x_n$ and disjoint subsets $I,J \subseteq [n]$, it holds:
$ P(X_i \geq x_i, \forall i \in I \cup J ) \leq P(X_i \geq x_i, \forall i \in I) P(X_j \geq x_j, \forall j \in J) $, and 
$ P(X_i \leq x_i, \forall i \in I \cup J ) \leq P(X_i \leq x_i, \forall i \in I) P(X_j \leq x_j, \forall j \in J) $.
\end{corollary}

The first inequality in \ref{Cor_NA_ProbabilityInequality} can be proved by taking function $f$ and $g$ to be indicator functions $f(X_i:i\in I)=1\{X_i\geq x_i\}$ and $g(X_j:j\in J)=1\{X_j \geq x_j\}$. The second equation can be derived similarly by taking the indicator function in the other direction.

Now, let’s come back and understand how can we use these definitions and lemmas in our problem. And for clarity, we include another concept Negative Dependent (ND), which is a special case of Negative Associated we mentioned above.

\begin{definition}[Negative Dependence (ND)] \label{Def_ND}
Random variables $X_1,…,X_n$ are said to be negatively dependent if both of the following two inequalities holds for any $x_1,…,x_n \in R$
$$ P( \bigcap_i X_i \geq x_i ) \leq \prod_i P(X_i \geq x_i) $$ 
$$ P( \bigcap_i X_i \leq x_i ) \leq \prod_i P(X_i \leq x_i)  $$
\end{definition}

Definition \ref{Def_ND} follows by simply taking the disjoint index set of $X_1,…,X_n$ as $1,…,n$ in Corollary \ref{Cor_NA_ProbabilityInequality}. This definition is also stated as Marginal probability Bounds \cite{Wajc217}.

With such definition, we can derive some nice properties that will be used latter \cite{Rita208}.

\begin{lem} \label{Lem_ND_2points}
Let $X_1,…,X_n$ be negatively dependent random variables, then:
\begin{itemize}
  \item If $f_1,…,f_n$ is a sequence of measurable functions which are all monotone non-decreasing (or all are monotone non-increasing), then $f_1(X_1),…,f_n(X_n)$ are also negatively dependent random variables.
  \item $E[X_1…X_n ] \leq E[X_1]…E[X_n]$, provided the expectation exist.
\end{itemize}
\end{lem}

The first point follows by applying Definition \ref{Def_ND} in the following way:
If  $f_1,…,f_n$ are all monotone non-decreasing functions, then
$ P( \bigcap_{i=1}^n (f(X_i)\leq f(x_i)) ) = P( \bigcap_{i=1}^n (X_i\leq x_i) ) \leq 
\prod_{i=1}^n P(X_i \leq x_i) = \prod_{i=1}^n P(f(X_i) \leq f(x_i)) $, and 
$ P( \bigcap_{i=1}^n (f(X_i)\geq f(x_i)) ) = P( \bigcap_{i=1}^n (X_i\geq x_i) ) \leq 
\prod_{i=1}^n P(X_i \geq x_i) = \prod_{i=1}^n P(f(X_i) \geq f(x_i)) $. We can also prove this similarly if $f_1,…,f_n$ are all monotone non-increasing functions.

The LFS of the second point can be written as 
$ E[X_1...X_n] = \int\int...\int P( \bigcap_{i=1}^n(X_i\geq x_i))dx_1dx_2...dx_n $,
while the RHS equals to 
$ E[X_1]...E[X_n] = \int P(X_1\geq x_1)dx_1 ... \int P(X_n\geq x_1)dx_n = \int\int...\int \prod_{i=1}^n P(X_i\geq x_i) dx_1dx_2...dx_n $,
and the inequality follows since $P( \bigcap_{i=1}^n(X_i\geq x_i))\leq P(X_i\geq x_i)$.

\begin{lem} \label{Lem_ND_ExpectationProduct}
Let $X_1,…,X_n$ be negatively dependent random variables, then:
$$  E[\exp(\lambda \sum_{i=1}^m X_i)] \leq \prod_{i=1}^m E[e^{\lambda X_i}]  $$
\end{lem}

Firstly, by applying the first point in Lemma \ref{Lem_ND_2points}, we know that $f_1(X_1),…,f_n(X_n)$ are also negatively dependent random variables. 
Then by applying the second point in Lemma \ref{Lem_ND_2points}, $E[f_1(X_1 )…f_n(X_n)] \leq E[f_1(X_1)]…E[f_n(X_n)] $
If $ \lambda \geq 0$, then we can take a non-decreasing function $ f_i(X_i) = e^{\lambda X_i}$ for each $i$, and the inequality in this lemma holds. 
Similarly, if $ \lambda \leq 0$, then we can take a non-increasing function $f_i(X_i) = e^{\lambda X_i}$, and the inequality will also holds. Actually, we say that $X_1,...X_n$ are acceptable if the inequality in lemma \ref{Lem_ND_2points} holds for any real $\lambda$ \cite{Rita208}. And NA implies acceptability if the Laplace transforms $E[e^{\lambda X_i}]$ are finite for all $i$.

We notice that the inequality in Lemma \ref{Lem_ND_ExpectationProduct} is exactly the relationship we want to prove for orthogonal random features. Therefore, our next step is to prove that orthogonal random features are negatively dependent, which is consistent with our intuition.

\begin{lem} \label{Lem_abs_ort}
$\vert{\omega_1^{ort}}^T Z\vert,...,\vert{\omega_n^{ort}}^T Z\vert$ are negatively dependent.
\end{lem}

From the definition of negative dependence, what we need to prove is
$ P( \bigcap_i (\vert{w_i^{ort}}^T Z\vert \leq \tilde{x}_i) ) \leq \prod_i P(\vert{w_i^{ort}}^T Z\vert \leq \tilde{x}_i) $, and $ P( \bigcap_i (\vert{w_i^{ort}}^T Z\vert \geq \tilde{x}_i) ) \leq \prod_i P(\vert{w_i^{ort}}^T Z\vert \geq \tilde{x}_i) $, where we use $ \tilde{x}_i$  to represent a different value than the original $x_i$, which should be $f^{-1}(x_i)$. We will illustrate how to prove the first inequality here since the other can be proved accordingly.

Firstly, we can decompose $w_i^{ort}=v_i l_i$, where $v_i^{ort}$ has unit length, and $l_i$ is taken independent from $v_i^{ort}$, which represents the length scalar.
So we need to prove 
$ P( \bigcap_i (\vert{v_i^{ort}}^T Z\vert \leq \frac{\tilde{x}_i}{l_i} ) ) \leq \prod_i P(\vert{v_i^{orhttps://www.overleaf.com/project/5e1343de08771b000145df67t}}^T Z\vert \leq \frac{\tilde{x}_i}{l_i}) $.

But actually since negatively dependence should holds for any $x_i \in R$, so it actually does not matters which scalar we use in the right hand side of each part of the probability inequality. So we will continue to use $x_i$ instead of $\frac{\tilde{x}_i}{l_i}$  in the following proof.

Proof for the cases when $x_j\geq 1$ or $x_j\leq 0$ is trivial, so we will only concentrate on the case when $0< x_j < 1$. Here, we can use a second trick for distribution transformation. We regard $v_1$, $v_2$, ..., $v_n$ as fixed, and $Z$ as a random rotation vector. Furthermore, we assume $\Vert Z\Vert_2=1$ for simplicity. Then the distribution of $\vert{v_i^{ort}}^T Z\vert$ will be equivalent to $e_1^T \frac{\vert g \vert}{{\Vert g \Vert}_2}=\frac{g_i}{{\Vert g \Vert}_2}$, where $g$ is a gaussian vector, and $g_i$ is the length of projection onto the $i^{th}$ coordinate.

So we need to prove $ P( \bigcap_i (\frac{g_i}{{\Vert g \Vert}_2}\leq x_i) ) \leq \prod_i P(\frac{g_i}{{\Vert g \Vert}_2}\leq x_i) $.
From the rule of conditional probability, the LFS can be transformed to $ P(\frac{g_1}{{\Vert g \Vert}_2}\leq x_1)P(\frac{g_2}{{\Vert g \Vert}_2}\leq x_2 \vert \frac{g_1}{{\Vert g \Vert}_2}\leq x_1)P(\frac{g_3}{{\Vert g \Vert}_2}\leq x_3 \vert (\frac{g_1}{{\Vert g \Vert}_2}\leq x_1)\cap (\frac{g_2}{{\Vert g \Vert}_2}\leq x_2) )... $. Therefore, it’s obvious that we only need to prove $P(\frac{g_i}{{\Vert g \Vert}_2}\leq x_i \vert \bigcap_{j=1}^{i-1} (\frac{g_j}{{\Vert g \Vert}_2}\leq x_j) ) \leq P(\frac{g_i}{{\Vert g \Vert}_2}\leq x_i)$ for each corresponding term.

We note that $\frac{g_j}{{\Vert g \Vert}_2}\leq x_j$ is equivalent to $\frac{{g_j}^2}{{\Vert g \Vert}_{2}^{2}} \leq {x_j}^2$, so for each $j<i$ we have ${g_j}^2 \leq {x_j}^2 {g_j}^2 + {x_j}^2 ({g_1}^2 + ... + {g_{i-1}}^2 + {g_{i+1}}^2 +...+{g_{n}}^2  ) $, which can be rewrite as $ {g_i}^2 \geq \frac{{g_j}^2}{{x_j}^2} - ({g_1}^2 + ... + {g_{i-1}}^2 + {g_{i+1}}^2 +...+{g_{n}}^2  ) $. We can also write from $\frac{g_i}{{\Vert g \Vert}_2}\leq x_i$ and derive $ {g_i}^2 \leq \frac{{x_i}^2}{(1-{x_i}^2)} ({g_1}^2 + ... + {g_{i-1}}^2 + {g_{i+1}}^2 +...+{g_{n}}^2  )  $.

Therefore, $P(\frac{g_i}{{\Vert g \Vert}_2}\leq x_i \vert \bigcap_{j=1}^{i-1} (\frac{g_j}{{\Vert g \Vert}_2}\leq x_j) ) = P({g_i}^2 \leq \frac{{x_i}^2}{(1-{x_i}^2)} ({g_1}^2 + ... + {g_{i-1}}^2 + {g_{i+1}}^2 +...+{g_{n}}^2  ) \vert \bigcap_{j=1}^{i-1} ( {g_i}^2 \geq \frac{{g_j}^2}{{x_j}^2} - ({g_1}^2 + ... + {g_{i-1}}^2 + {g_{i+1}}^2 +...+{g_{n}}^2  ) )  ) \leq  P({g_i}^2 \leq \frac{{x_i}^2}{(1-{x_i}^2)} ({g_1}^2 + ... + {g_{i-1}}^2 + {g_{i+1}}^2 +...+{g_{n}}^2  )) = P(\frac{g_i}{{\Vert g \Vert}_2 }\leq x_i) $, which finished our proof of negative dependence.

\begin{thm} [Strong Concentration] \label{Thm_StrongConcentration}

Suppose function $f: \mathcal{R}^{+} \mapsto \mathcal{R}$ can be decomposed as $f=f^{+} + f^{-}$, where $f^{+}$ and $f^{-}$ represent monotone increasing and decreasing part respectively. If $f^{+}(\vert \omega_i^T Z \vert) \in [a_i^{+},b_i^{+}]$ and $f^{-}(\vert \omega_i^T Z \vert) \in [a_i^{-},b_i^{-}]$ a.s., then $\hat{F}_m^{ort}(Z)=\frac{1}{m}\sum_{i=1}^m f(\vert {\omega_i^{ort}}^T Z \vert)$ satisfies upper tail bound:
$P(|\hat{F}_m^{ort}(Z) - F_f(Z)| \geq t)
 \leq 2\exp(-\frac{m^2 t^2}{2\sum_i {(b_i^{+}-a_i^{+})}^2})+2\exp(-\frac{m^2 t^2}{2\sum_i{(b_i^{-}-a_i^{-})}^2})$ a.s.. Furthermore, if $f$ is non-negative and monotone increasing (or decreasing), then orthogonal random features will provide tighter strong concentration bound than i.i.d random features: $P(\hat{F}_m^{ort} \geq a) \leq P(\hat{F}_m^{iid} \geq a)$, $P(\hat{F}_m^{ort} \leq a) \leq P(\hat{F}_m^{iid} \leq a)$, $\forall a>0$.

\end{thm}

Firstly, we decompose the estimator into increasing and decreasing parts: $\hat{F}_m^{ort}(Z) = \frac{1}{m} \sum_{i=1}^m f(|{\omega_i^{ort}}^T Z|) = \frac{1}{m}
\sum_{i=1}^m (f^{+}(|{\omega_i^{ort}}^T Z|)+ f^{-}(|{\omega_i^{ort}}^T Z|)) = {\hat{F}_m^{+,ort}}(Z)+{\hat{F}_m^{-,ort}}(Z)$, which are ND respectively. By applying Chernoff–Hoeffding inequalities for ND random variables \cite{Dev196}, we have:
$P(|\hat{F}_m^{+,ort}(Z) - F_{f^{+}}(Z)| \geq t)\leq 
2\exp(-\frac{m^2 t^2}{2\sum_i {(b_i^{+}-a_i^{+})}^2})$,
 $P(|\hat{F}_m^{-,ort}(Z) - F_{f^{-}}(Z)| \geq t) \leq 
2\exp(-\frac{m^2 t^2}{2\sum_i {(b_i^{-}-a_i^{-})}^2})$ a.s.. 
Therefore, $P(|\hat{F}_m^{ort}(Z) - F_f(Z)| \geq t) = P(|\hat{F}_m^{+,ort}(Z)+\hat{F}_m^{-,ort}(Z) - F_{f^{+}}(Z)-F_{f^{-}}(Z)| \geq t)
 \leq P(|\hat{F}_m^{+,ort}(Z) - F_{f^{+}}(Z)| + |\hat{F}_m^{-,ort}(Z)-F_{f^{-}}(Z)| \geq t) \leq P(|\hat{F}_m^{+,ort}(Z) - F_{f^{+}}(Z)|\geq \frac{t}{2})+ P(|\hat{F}_m^{-,ort}(Z) - F_{f^{-}}(Z)|\geq \frac{t}{2}) \leq 2\exp(-\frac{m^2 t^2}{2\sum_i {(b_i^{+}-a_i^{+})}^2})+2\exp(-\frac{m^2 t^2}{2\sum_i{(b_i^{-}-a_i^{-})}^2})$ a.s..

From Lemma \ref{Lem_NA_ExpectationProductInequality}, Lemma \ref{Lem_ND_2points} and Lemma \ref{Lem_abs_ort}, we can derive directly that if the function $f$ is monotone increasing (or decreasing) in $\vert \omega_i^T Z \vert$, then ND of $\vert{\omega_1^{ort}}^T Z\vert,...,\vert{\omega_n^{ort}}^T Z\vert$ implies $E[\exp(\lambda \sum_{i=1}^m X_i^{ort})] \leq \prod_{i=1}^m E[e^{\lambda X_i^{ort}}] = \prod_{i=1}^m E[e^{\lambda X_i^{iid}}] $, $\forall \lambda \in \mathcal{R}$, which is exactly the inequality for proving orthogonal random features have better strong concentration bound than independent random features derived after Lemma \ref{Lem_ExtendedMarkovInequality}.
