# Supplementary material for: Demystifying Orthogonal Monte Carlo and Beyond
Source: arXiv:2005.13590 source file (2020-05-27)
Supplement: Supplementary file 2 [file appendix.tex]

\section*{OLD APPENDIX: Demystifying Orthogonal Monte Carlo and Beyond}

\subsection{Main Proof of Theorem \ref{mainlemma}}
Denote $\eta_1^{\text{iid}},...,\eta_s^{\text{iid}}$ as independent and identical samples from standard normal distribution $N(0,I_d)$ and $\eta_1^{\text{ort}},...,\eta_s^{\text{ort}}$ as orthogonal and identical samples from standard normal distribution. 
Let $Y_i^{\text{iid}} = \Sigma^{-1}Vz(\eta_i^{\text{iid}})z(\eta_i^{\text{iid}})^*V^*\Sigma^{-1}$ and $Y_i^{\text{ort}} = \Sigma^{-1}Vz(\eta_l^{\text{ort}})z(\eta_i^{\text{ort}})^*V^*\Sigma^{-1}$. We further denote $Z^{\text{ort}} = \frac{1}{s}\sum\limits_ {i=1}^s Y_i^{\text{ort}}-\Sigma^{-1}VKV^*\Sigma^{-1}$ and $Z^{\text{iid}} = \frac{1}{s}\sum\limits_{i=1}^s Y_i^{\text{iid}}-\Sigma^{-1}VKV^*\Sigma^{-1}$. Note that for identical independent setting, we have 
\begin{align}\label{iid_inequality}
    \mathbb{P}(\|Z^{\text{iid}}\|_2\geq \Delta) \leq 16s_\lambda(K) \text{exp}{(\frac{-3s\Delta^2}{8n_\lambda})}.
\end{align}
We show that orthogonal samples can give the same approximation with at least the same probability as unstructured approach, but for a smaller number of random features. The idea of proof is to show $P(\|\frac{1}{s}\sum\limits_{i=1}^s Y_i^{\text{ort}}-\Sigma^{-1}VKV^*\Sigma^{-1}\|_2\geq \Delta)$ is less than or equal to a shrinking coefficient $C$ (less than $1$) multiplied by the right hand side of \eqref{iid_inequality}. With that, we have 
\begin{eqnarray}
\mathbb{P}(\|\frac{1}{s}\sum\limits_{i=1}^s Y_i^{\text{ort}}-\Sigma^{-1}VKV^*\Sigma^{-1}\|_2\geq 
\Delta)\leq\notag\\
 16Cs_\lambda(K)\text{exp}(\frac{-3s\Delta^2}{8n_\lambda}).
\end{eqnarray}
Therefore, under orthogonal sampling, $\frac{8}{3}\Delta^{-2}n_\lambda \ln{(16Cs_\lambda(K)/\rho)} \le \frac{8}{3}\Delta^{-2}n_\lambda \ln{(16s_\lambda(K)/\rho)}$) under identical independent sampling. 

First, it is not hard to see
\begin{eqnarray}
\mathbf{E}[Y_i^{\text{iid}}]=\mathbf{E}[Y_i^{\text{ort}}] = \Sigma^{-1}VKV^*\Sigma^{-1}.
\end{eqnarray}
and
\begin{align}
 \|Y_i^{\text{iid}}\|_2 &=  \|Y_i^{\text{ort}}\|_2\notag\\
 &= \text{Tr}(\Sigma^{-1}Vz(\eta_i^{\text{ort}})z(\eta_i^{\text{ort}})^*V^*\Sigma^{-1})\notag\\
&=z(\eta_i^{\text{ort}})^*(K+\lambda I_n)^{-1}z(\eta_i^{\text{ort}})\notag\\
&\le  \int p(\eta_i^{\text{ort}})z(\eta_i^{\text{ort}})^*(K+\lambda I_n)^{-1}z(\eta_i^{\text{ort}})d\eta_i^{\text{ort}} \notag\\
&  =  \int p(\eta_i^{\text{iid}})z(\eta_i^{\text{iid}})^*(K+\lambda I_n)^{-1}z(\eta_i^{\text{iid}})d\eta_i^{\text{iid}}\notag\\
& =\text{Tr}((K+\lambda I_n)^{-1}K)=s_\lambda(K).
\end{align}
According to Proposition 5 of \cite{AKMM2}).
\begin{eqnarray}
(Y_i^{\text{ort}})^2\textbf{}&=\frac{\tau(\eta_i^{ort})}{p(\eta_i^{ort})}\Sigma^{-1}Vz(\eta_i^{\text{ort}})z(\eta_i^{\text{ort}})^*V^*\Sigma^{-1}\notag\\
&=\frac{\tau(\eta_i^{ort})}{p(\eta_i^{ort})}Y_i^{\text{ort}} = \frac{n_\lambda \tau(\eta_i^{ort})}{\tilde{\tau}(\eta_i^{ort})}Y_i^{\text{ort}}\preceq Y_i^{\text{ort}}
\end{eqnarray}
To show
$\mathbb{P}(\|\frac{1}{s}\sum\limits_{i=1}^s Y_i^{\text{ort}}-\Sigma^{-1}VKV^*\Sigma^{-1}\|_2\geq \Delta)\leq 16Cs_\lambda(K)\text{exp}(\frac{-3s\Delta^2}{8n_\lambda})$, we apply Markov equality with a fixed positive number $\theta$ such that 
\begin{align}
\mathbb{P}(\|Z^{\text{ort}}\|_2\geq \Delta)&=\mathbb{P}\{e^{\theta \|Z^{\text{ort}}\|_2} \geq e^{\theta t}\}\notag\\
&\leq e^{-\theta t} \mathbb{E}[e^{\theta \|Z^{\text{ort}}\|_2}]=e^{-\theta t} \mathbb{E}[e^{\|\theta Z^{\text{ort}}\|_2}].
\end{align}
The first identity holds because $a\to e^{\theta a}$ is a monotone increasing function, so the event does not change under the mapping. The second relation is Markov's inequality. The last holds because the maximum eigenvalue is a positive-homogeneous map. To control the exponential, 
note that 
\begin{align}
e^{||\theta Z^{\text{ort}}||} = ||e^{\theta Z^{\text{ort}}}||\leq \text{Tr}(e^{\theta Z^{\text{ort}}}).
\end{align}
The first identity depends on the Spectral Mapping Theorem and the fact that the exponential function is increasing. The inequality follows because the exponential of an Hermitian matrix is positive definite and the last follows because the maximum eigenvalue of a positive-definite matrix is dominated by the trace. Combine the latter two displays and take an infimum to achieve the tightest possible bound,  
\begin{align}
\mathbb{P}(||Z^{\text{ort}}||\geq t)&\leq e^{-\theta t}\mathbf{E}[\text{Tr}e^{\theta Z^{\text{ort}}}],\\
\mathbb{P}(||Z^{\text{ort}}||\geq t)&\leq \inf_{\theta>0} e^{-\theta t}\mathbf{E}[\text{Tr}(e^{\theta Z^{\text{ort}}})].
\end{align}
Note that the above derivation still works for $Z^{\text{iid}}$, i.e. 
\begin{align}
\mathbb{P}(||Z^{\text{iid}}||\geq t)&\leq \inf_{\theta>0} e^{-\theta t}\mathbf{E}[\text{Tr}(e^{\theta Z^{\text{iid}}})].\label{iid_mgf}
\end{align}
Moreover, the right hand side of \eqref{iid_mgf} is bounded by $16s_\lambda(K)\text{exp}(\frac{-3s\Delta^2}{8n_\lambda})$ as the derivation above just follows the initial step of proof of Bernstein concentration inequality. Therefore, if we can show that $  \mathbf{E}[\text{Tr}(e^{\theta Z^{\text{ort}}})]< \mathbf{E}[\text{Tr}(e^{\theta Z^{\text{iid}}})]$, we will have $P(\|Z^{\text{ort}}\|_2\geq \Delta)\leq C\cdot 16s_\lambda(K)\text{exp}(\frac{-3s\Delta^2}{8n_\lambda})$ with $C\leq 1$ to conclude the proof. 

Therefore, we only need to show $\mathbf{E}[\text{Tr}(e^{\theta Z^{\text{ort}}})]< \mathbf{E}[\text{Tr}(e^{\theta Z^{\text{iid}}})]$. Without loss of generality, we assume that $\theta=1$ by absorbing the parameter into the random matrices. Note that 
\begin{align}
&\mathbf{E}\big[\text{Tr}(e^{Z^{\text{ort}}})\big]\\
=&\mathbf{E}\Big[\text{Tr}\big(\text{exp}( \frac{1}{s}\sum\limits_ {i=1}^s Y_i^{\text{ort}}-\Sigma^{-1}VKV^*\Sigma^{-1})\big)\Big]\\
=&\mathbf{E}\bigg[\text{Tr}\Big(\text{exp}\big( \Sigma^{-1}V \big(\frac{1}{s}\sum\limits_ {i=1}^s z(\eta_i^{\text{ort}})z(\eta_i^{\text{ort}})^*-K\big)V^*\Sigma^{-1}\big)\Big)\bigg]\\
<& \mathbf{E}\bigg[\text{Tr}\Big(\text{exp}\big( \Sigma^{-1}V \big(\frac{1}{s}\sum\limits_ {i=1}^s z(\eta_i^{\text{iid}})z(\eta_i^{\text{iid}})^*-K\big)V^*\Sigma^{-1}\big)\Big)\bigg]\\
=&\mathbf{E}\big[\text{Tr}(e^{Z^{\text{iid}}})\big].
\end{align}

It remains to show that 
\begin{align}\label{kernelmethod1_key}
&\mathbf{E}\bigg[\text{Tr}\Big(\text{exp}\big( \Sigma^{-1}V \big(\frac{1}{s}\sum\limits_ {i=1}^s z(\eta_i^{\text{ort}})z(\eta_i^{\text{ort}})^*-K\big)V^*\Sigma^{-1}\big)\Big)\bigg]\notag \\
< &\mathbf{E}\bigg[\text{Tr}\Big(\text{exp}\big( \Sigma^{-1}V \big(\frac{1}{s}\sum\limits_ {i=1}^s z(\eta_i^{\text{iid}})z(\eta_i^{\text{iid}})^*-K\big)V^*\Sigma^{-1}\big)\Big)\bigg]
\end{align}

Let $M_{ort} = \Sigma^{-1}V \big(\frac{1}{s}\sum\limits_ {i=1}^s z(\eta_i^{\text{ort}})z(\eta_i^{\text{ort}})^*-K\big)V^*\Sigma^{-1}$, $M_{iid}= \Sigma^{-1}V \big(\frac{1}{s}\sum\limits_ {i=1}^s z(\eta_i^{\text{iid}})z(\eta_i^{\text{iid}})^*-K\big)V^*\Sigma^{-1}$.

Another way to prove the theorem is to show that 
\begin{align}\label{kernelmethod2_key}
\|\mathbf{E}M_{ort}^2\|\leq \|\mathbf{E}M_{iid}^2\|
\end{align}
because with that, we have 
\begin{align}\label{kernelmethod2}
\mathbb{P}(||Z^{\text{ort}}||\geq t)&\leq \inf_{0<\theta<3/L}de^{-\theta t}\text{exp}(\frac{\theta^2}{1-\theta L/3}\|\mathbf{E}M_{ort}^2\|)\notag \\
&\leq \inf_{0<\theta<3/L}de^{-\theta t}\text{exp}(\frac{\theta^2}{1-\theta L/3}\|\mathbf{E}M_{iid}^2\|)
\end{align}
where $\|M_{ort}\|\leq L$,$\|\Sigma^{-1}V \big( z(\eta_i^{\text{iid}})z(\eta_i^{\text{iid}})^*-\frac{1}{s}K\big)V^*\Sigma^{-1}\|\leq L$ (I have not verify these inequalities yet, which is an essential step in having the first inequality holds true of \eqref{kernelmethod2}). The RHS of inequalities \eqref{kernelmethod2} is smaller than or equal to $16s_\lambda(K) \text{exp}{(\frac{-3s\Delta^2}{8n_\lambda})}$ based on the original proof of the Bernstein inequality. Hence, it will conclude the proof if we have $\|\mathbf{E}M_{ort}^2\|\leq \|\mathbf{E}M_{iid}^2\|$. 

For now, we have two possible ideas to prove the theoerm. Either we prove \eqref{kernelmethod1_key} or prove \eqref{kernelmethod2_key} we can finish the proof of the theorem. 

For now, we can successfully prove
\begin{align}
&\Tr(\mathbf{E}\big(\frac{1}{s}\sum\limits_ {i=1}^s z(\eta_i^{\text{ort}})z(\eta_i^{\text{ort}})^*-K\big)^2)<\notag\\ &\Tr(\mathbf{E}\big(\frac{1}{s}\sum\limits_ {i=1}^s z(\eta_i^{\text{iid}})z(\eta_i^{\text{iid}})^*-K\big)^2)
\end{align}
by using the result $\mathbf{E}[\cos{(n_1\eta_1^{\text{ort}}+n_2\eta_2^{\text{ort}})^Tz}]<\mathbf{E}[\cos{(n_1\eta_1^{\text{iid}}+n_2\eta_2^{\text{iid}})^Tz}]$.
